# Supplementary material for: Observation of quasi bound states in open quantum wells of cesiated p-doped GaN surfaces
Source: arXiv:2503.22393 source file (2026-03-02)
Supplement: Supplementary file 1 [file 2025-03-28-Supp_Mat_BBr.pdf]

# Observation of quasi bound states in open quantum wells of cesiated p-doped GaN surfaces - Supplemental Material

Mylène Sauty<sup>1,2</sup>, Jean-Philippe Banon<sup>1,3</sup>, Nicolas M. S. Lopes<sup>1</sup>,  
Tanay Tak<sup>4</sup>, James S. Speck<sup>4</sup>, Claude Weisbuch<sup>1,4</sup>, Jacques Peretti<sup>1</sup>

<sup>1</sup>*Laboratoire de Physique de la Matière Condensée, CNRS,  
Ecole polytechnique, Institut Polytechnique de Paris, 91120 Palaiseau, France*

<sup>2</sup>*Service de Physique de l'État condensé (SPEC),  
Université Paris-Saclay, CEA-CNRS, F-91191, Gif-sur-Yvette, France*

<sup>3</sup>*Laboratoire Charles Fabry, Institut d'Optique Graduate School,  
CNRS, Université Paris-Saclay, 91127 Palaiseau, France*

<sup>4</sup>*Materials Department, University of California, Santa Barbara, California 93106, USA*  
(Dated: March 28, 2025)

In this Supplemental Material, we describe in Section I the theoretical model which we have used in the article to determine the electron local density of states (LDOS). We first describe in Sec. IA the framework of the effective mass approximation to describe wave functions supported both inside and outside the semiconductor and discuss the relevance and limitations of such a model for describing low energy eigenstates. The aim of this first subsection is to set the stage and discuss the approximations. Section IB is then devoted to the implementation of Green's function in the effective mass framework. In an open system, like the one studied here in the context of a photoemission experiment, the electron Green's function at a given energy and satisfying an outgoing radiation condition is the ideal tool as (i) it directly describes an infinite system (and thus avoid the cumbersome use of an arbitrary quantization box for the wave functions), and (ii) its imaginary part is directly proportional to the local density of states. Determining the Green's function requires the knowledge of the band bending electrostatic potential. Section IC is devoted to the non-linear Poisson equation for the electrostatic potential both in the quantum setting where the charge densities are determined from the quantum local density of states, and in the semi-classical setting. We show that the semi-classical approximation of the charge density is sufficient to determine the electrostatic potential in our case.

Details of the numerical implementation for computing the Green's function and the electrostatic potential are given in Section II.

Finally, in Section III, we comment works reporting experimental observations of the resonant states from the BBR of cesiated GaAs.

## I. THEORETICAL MODEL

### A. Conduction and valence band states

In a homogeneous crystalline semiconductor the eigenstates of the single electron Hamiltonian are given by Bloch waves of the form  $\psi_{\mathbf{k}}^{(v)}(\mathbf{r}) = u_{v,\mathbf{k}}(\mathbf{r}) \exp(i\mathbf{k} \cdot \mathbf{r})/L^{3/2}$  and  $\psi_{\mathbf{k}}^{(c)}(\mathbf{r}) =$

$u_{c,\mathbf{k}}(\mathbf{r}) \exp(i\mathbf{k} \cdot \mathbf{r})/L^{3/2}$ , where  $u_{v,\mathbf{k}}$  and  $u_{c,\mathbf{k}}$  are lattice-periodic functions. The length  $L$  denotes here the size of a sufficiently large quantization box with Born-von Karman boundary conditions. For a doped and cesiated semiconductor with a band bending near the surface at  $z = 0$  and a negative electron affinity, the eigenstates of the Hamiltonian are modified. Instead of Bloch waves, we may assume the states at energy  $\epsilon$  to have the form

$$\psi_{\epsilon,\mathbf{p}}^{(c,v)}(\mathbf{r}) = \tilde{u}_{c,v}(\mathbf{r}) \chi_{\epsilon,\mathbf{p}}^{(c,v)}(\mathbf{r}), \quad (1)$$

known as the effective mass approximation [1]. Here and in the following, the indices or superscripts  $(c, v)$  must be understood as related to quantities for the conduction or the valence band, respectively. The functions  $\tilde{u}_v$  and  $\tilde{u}_c$  are equal to the Bloch cell functions  $u_v \equiv u_{v,\mathbf{k}=\mathbf{0}}$  and  $u_c \equiv u_{c,\mathbf{k}=\mathbf{0}}$ , respectively, inside the material ( $z < 0$ ) and both functions are equal to 1 outside the material ( $z > 0$ ). Note that we choose the Bloch cell functions for  $\mathbf{k} = \mathbf{0}$  independently for all states since we are primarily interested in a regime close to the band edges where the cell functions do not vary much with  $\mathbf{k}$ . The cell functions are assumed to be normalized as follows

$$\frac{1}{|\Omega_{\text{cell}}|} \int_{\Omega_{\text{cell}}} |u_{c,v}(\mathbf{r})|^2 d^3r = 1, \quad (2)$$

where  $\Omega_{\text{cell}}$  denotes the unit cell of the crystal. The envelope functions  $\chi_{\epsilon,\mathbf{p}}^{(c,v)}$  satisfy the effective mass Schrödinger equations

$$-\frac{\hbar^2}{2} \nabla \cdot \left[ \frac{\nabla \chi_{\epsilon,\mathbf{p}}^{(c,v)}}{m_{c,v}} \right] + V_{c,v} \chi_{\epsilon,\mathbf{p}}^{(c,v)} = \epsilon \chi_{\epsilon,\mathbf{p}}^{(c,v)}. \quad (3)$$

Here  $\mathbf{p}$  is a degeneracy index for the eigenfunctions corresponding to the wave vector component in the  $(x, y)$  plane of the surface as will be clarified below. We make the reasonable assumption that the states in the valence band are restricted to occupy the volume of the semiconductor only and strictly vanish outside in the vacuum. Equation (3) for the valence band thus holds for  $z < 0$  supplemented with a homogeneous Dirichlet boundary condition at the surface  $z = 0$ , i.e.,  $\chi_{\epsilon,\mathbf{p}}^{(v)}|_{z=0} = 0$ . The functions  $m_v = -m_h < 0$  and  $m_c$  are  $z$ -dependent effective masses of the electron in the valence band and

in the conduction-vacuum band, respectively. The valence band effective mass  $m_v = -m_h$  will be constant inside the semiconductor and the conduction band effective mass  $m_c$  will take the constant value of the bulk conduction band electron effective mass  $m_e$  inside the semiconductor, and the free electron mass  $m_0$  in the vacuum. The potentials  $V_v$  and  $V_c$  are the valence and conduction potentials due to the band bending inside the semiconductor. Outside the semiconductor  $V_c$  takes the value of the vacuum level  $E_{\text{vac}}$ . In other words, we have

$$V_v(z) = E_v(z) \quad \text{defined only for } z < 0, \quad (4a)$$

$$V_c(z) = E_c(z) + (E_{\text{vac}} - E_c(z))\Theta(z), \quad (4b)$$

where  $\Theta$  is the Heaviside step function. The band profiles  $E_v(z)$  and  $E_c(z)$  inside the semiconductor are determined by solving self-consistently the Poisson equation where the charge density is given by a semi-classical expression and a given doping concentration. These equations are supplemented by a Dirichlet boundary condition for the electrostatic potential at the surface by pinning the Fermi level to be at mid-gap at the surface, and by a homogeneous Neumann boundary condition sufficiently far from the surface inside the bulk of the semiconductor where the electrostatic is expected to reach a constant asymptotic value (see Section IC for more details).

The equations for the envelope functions being invariant along the  $x$  and  $y$  variables, we can look for solutions to Eq. (3) in the form

$$\chi_{\epsilon, \mathbf{p}}^{(c,v)}(\mathbf{r}) = \frac{\exp(i \mathbf{p} \cdot \mathbf{r}_{\parallel})}{L} \bar{\chi}_{\epsilon, p}^{(c,v)}(z). \quad (5)$$

Here  $L$  is an arbitrary, sufficiently large, size of a square quantization surface in the  $(x, y)$ -plane, and  $\mathbf{p}$  is a wave vector in the  $(x, y)$ -plane, of the form  $\mathbf{p} = p_x \mathbf{e}_x + p_y \mathbf{e}_y$  with  $p_x = 2\pi n_x/L$ ,  $p_y = 2\pi n_y/L$  (with  $n_x$  and  $n_y \in \mathbb{Z}$ ). Inserting the expression in Eq. (5) into the Schrödinger Eq. (3), it follows that the  $z$ -depend factor of the wave function satisfies

$$-\frac{\hbar^2}{2} \frac{d}{dz} \left[ \frac{1}{m_{c,v}} \frac{d \bar{\chi}_{\epsilon, p}^{(c,v)}}{dz} \right] + \left[ V_{c,v} + \frac{\hbar^2 p^2}{2m_{c,v}} \right] \bar{\chi}_{\epsilon, p}^{(c,v)} = \epsilon \bar{\chi}_{\epsilon, p}^{(c,v)}, \quad (6)$$

where  $p^2 = p_x^2 + p_y^2$ . Note that in view of Eq. (6), the functions  $\bar{\chi}_{\epsilon, p}^{(c,v)}$  only depend on the norm of  $\mathbf{p}$  and not specifically on its direction, and which is a consequence of the invariance of the effective mass problem by rotations around the  $z$ -axis.

In view of the proposed effective mass model, Eq. (3), the coupling between the (quasi) Bloch wave inside the material and the wave function outside is assumed to be given by the continuity of the envelope function inside the material to the wave function in vacuum, and a jump relation for the derivative of the envelope function inside

the material and the wave function in vacuum due to the jump of effective mass. This is encoded in the form taken by the kinetic energy operator. This is of course only approximate since the true wave function (hence including the periodic part of the Bloch function) should be continuous as well as its derivative at the interface. The specific form of the kinetic energy operator shown in Eq. (3) originates from the continuity of the electron flux in a position dependent effective mass material and is commonly used for the modeling of heterostructures [2, 3]. However, this assumption is strictly speaking valid only for heterostructures involving materials with similar Bloch wave functions on both sides of the interface [4]. Although its validity can be questioned in the case of the interface between a semiconductor and vacuum, Eq. (3) is also encountered in this case, in particular for the modeling of low energy photoemission [5].

As a rule of thumb, we expect our model to be satisfactory in a regime where the typical de Broglie wavelength of the electron associated to the envelope function,  $\lambda_{\text{dB}}$ , is large compared to the lattice constants of the semiconductor crystal,  $\lambda_{\text{dB}} \gg a, c$ . The de Broglie wavelength being dependent on the electron energy and on the effective mass, via  $E - V = \hbar^2 k_{\text{dB}}^2 / 2m$ , with  $k_{\text{dB}} = 2\pi / \lambda_{\text{dB}}$ , we find the following criterion on the electron energy to fall within the aforementioned regime:  $k_{\text{dB}}^2(E) = 2m(E - V) / \hbar^2 \ll (2\pi / \max(a, c))^2$ , in other words the typical wave number in the semiconductor or in vacuum at energy  $E$  should be small compared with the size of the Brillouin zone. In view of the electron effective mass in the semiconductor being smaller than the mass of the electron in vacuum, and that in the NEA configuration  $E - E_{\text{vac}}$  is typically larger than  $E - V_{\text{bulk}}$ , the criterion is essentially constrained from the vacuum side, i.e.,  $2m_0(E - E_{\text{vac}}) / \hbar^2 \ll (2\pi / c)^2$ . This typically yields  $E - E_{\text{vac}} \ll 5.6$  eV for GaN, which is a reasonable bound considering that the near band gap low energy photoemission experiment typically operates from  $E - E_{\text{vac}} = 0$  to a few eV.

## B. Effective mass Green's function

An efficient way to estimate the local density of states is from the Green's function thanks to the general relation [6]

$$\text{LDOS}(\mathbf{r}, E) = -\frac{1}{\pi} \text{Im } \mathcal{G}(\mathbf{r}, \mathbf{r}, E). \quad (7)$$

Here  $\mathcal{G}(\mathbf{r}, \mathbf{r}', E)$  denotes the full Green's function of the entire open system at energy  $E$  between a source point  $\mathbf{r}'$  and an observation point  $\mathbf{r}$  and subjected to outgoing radiation condition. The full Green's function accounting for the crystalline structure of the semiconductor is difficult to determine in practice. For low energy photoemission, in a regime for which the typical de Broglie wavelength of the electron is large compared with the lattice size, we may rather be interested in an effective Green's

function which somewhat homogenizes the crystal lattice. For an energy  $E$  larger than the vacuum level, the spectral representation of the Green's function  $\mathcal{G}(\mathbf{r}, \mathbf{r}', E)$  can be approximated by

$$\mathcal{G}(\mathbf{r}, \mathbf{r}', E) = \sum_{\epsilon, \mathbf{p}} \frac{\psi_{\epsilon, \mathbf{p}}^{(c)}(\mathbf{r}) \psi_{\epsilon, \mathbf{p}}^{(c)*}(\mathbf{r}')}{E - \epsilon + i0}, \quad (8)$$

where only the contribution from states in the conduction-vacuum band need to be accounted for. In the effective mass approximation, the eigenstates  $\psi_{\epsilon, \mathbf{p}}^{(c)}$  are given by Eq. (1). Inserting Eq. (1) into Eq. (8) we obtain

$$\mathcal{G}(\mathbf{r}, \mathbf{r}', E) = \tilde{u}_c(\mathbf{r}) \tilde{u}_c^*(\mathbf{r}') G^{(c)}(\mathbf{r}, \mathbf{r}', E), \quad (9)$$

with

$$G^{(c)}(\mathbf{r}, \mathbf{r}', E) = \sum_{\epsilon, \mathbf{p}} \frac{\chi_{\epsilon, \mathbf{p}}^{(c)}(\mathbf{r}) \chi_{\epsilon, \mathbf{p}}^{(c)*}(\mathbf{r}')}{E - \epsilon + i0}. \quad (10)$$

Note that the product of cell functions  $\tilde{u}_c(\mathbf{r}) \tilde{u}_c^*(\mathbf{r}')$  can be factorized out of the sum in Eq. (9) since we have made the approximation that the cell functions do not depend

much on the wave vector  $\mathbf{p}$  and the energy  $\epsilon$  provided the energy remains close to the band edge. Equation (9) can be interpreted as follows. The full, crystalline, Green's function in the effective mass approximation,  $\mathcal{G}$ , can be seen as the Green's function for a homogeneous medium,  $G^{(c)}$ , weighted at the source and the observation points by the local cell function. By inspection of Eq. (10), it is clear that the Green's function for the homogeneous medium,  $G^{(c)}$ , is precisely the Green's function associated with Eq. (3), i.e.,

$$\frac{\hbar^2}{2} \nabla \cdot \left[ \frac{\nabla G^{(c)}}{m_c} \right] (\mathbf{r}, \mathbf{r}', E) + (E - V_c) G^{(c)}(\mathbf{r}, \mathbf{r}', E) = \delta(\mathbf{r} - \mathbf{r}'), \quad (11)$$

and subjected to outgoing radiation condition.

As a consequence of the translation invariance of the problem for the envelope functions in the  $(x, y)$ -plane, the Green's function  $G^{(c)}$  depends only on the difference of in-plane positions  $\mathbf{r}_{\parallel} - \mathbf{r}'_{\parallel}$ , and on the coordinates  $z$  and  $z'$ , i.e., we may rather use the notation  $G^{(c)}(\mathbf{r}, \mathbf{r}', E) \equiv G^{(c)}(\mathbf{r}_{\parallel} - \mathbf{r}'_{\parallel}, z, z', E)$ . By taking the Fourier transform over the  $x$  and  $y$  variables in Eq. (11) we obtain the following equation

$$\frac{\hbar^2}{2} \frac{d}{dz} \left[ \frac{1}{m_c} \frac{d\bar{G}^{(c)}}{dz} \right] (\mathbf{p}, z, z', E) + \left[ E - V_c - \frac{\hbar^2 p^2}{2m_c} \right] \bar{G}^{(c)}(\mathbf{p}, z, z', E) = \delta(z - z'), \quad (12)$$

for the Fourier coefficient  $\bar{G}^{(c)}(\mathbf{p}, z, z', E)$  defined by

$$G^{(c)}(\mathbf{r}_{\parallel}, z, z', E) = \int_{\mathbb{R}^2} \bar{G}^{(c)}(\mathbf{p}, z, z', E) \exp(i\mathbf{p} \cdot \mathbf{r}_{\parallel}) \frac{d^2 p}{(2\pi)^2}. \quad (13)$$

Equation (13) is known as the Weyl's representation, or angular spectrum, of the Green's function [7]. Also note that Eq. (12) corresponds to the Green's function associated to the Schrödinger equation (6) for the  $z$ -dependent factor of the envelope function for a given in-plane wave vector. Consistently with the above development on the Green's function, the local density of states in the conduction-vacuum band is approximated by

$$\begin{aligned} \text{LDOS}(\mathbf{r}, E) &= |\tilde{u}_c(\mathbf{r})|^2 \text{LDOS}^{(c)}(\mathbf{r}, E) \\ &= -\frac{|\tilde{u}_c(\mathbf{r})|^2}{\pi} \text{Im } G^{(c)}(\mathbf{r}, \mathbf{r}, E), \end{aligned} \quad (14)$$

where the second equality is a defining equality for the effective mass local density of states  $\text{LDOS}^{(c)}(\mathbf{r}, E)$ . The latter can be interpreted as a local density of states spatially smoothed over the lattice, i.e., that its typical spatial length scale is given by the de Broglie wavelength of the underlying envelope functions. The system being invariant by translation in the  $(x, y)$ -plane for the effective mass LDOS, we can define its associated two-

dimensional Fourier transform in a similar way as for the Green's function, which gives

$$\text{LDOS}^{(c)}(\mathbf{p}, z, E) = -\frac{1}{\pi} \text{Im } \bar{G}^{(c)}(\mathbf{p}, z, z, E). \quad (15)$$

The Fourier component of the LDOS,  $\text{LDOS}^{(c)}(\mathbf{p}, z, E)$ , thus measures the number of states per unit energy and unit volume, with in-plane wave-vector  $\mathbf{p}$ , around point  $z$  and energy  $E$ . In the article, for the interpretation of the energy distribution of the photo-electrons, the local density of states for vanishing in plane wave-vector  $\mathbf{p} = \mathbf{0}$  is of particular interest. Indeed, after relaxation, the excited electrons tend to accumulate near vanishing in-plane wave-vectors to minimize their energy. Figure 3(a) in the article presents a map of the local density of states for vanishing wave-vector as a function of  $z$  and  $E$  for a potential profile representative of the experimental sample, obtained by computing numerically  $\bar{G}^{(c)}(\mathbf{p}, z, z', E)$ . The numerical scheme used to solve Eq. (12) for  $\bar{G}^{(c)}(\mathbf{p}, z, z', E)$  is described in details in Sec. II A.

### C. Band bending profile

The band bending profile in the vicinity of the surface inside the semiconductor is determined by the electrostatic potential  $\phi$  resulting from the inhomogeneous charge distribution. In a p-doped semiconductor the charge distribution is composed of holes in the valence band and of the ionized acceptors. The Poisson equation giving the electrostatic potential reads

$$-\nabla \cdot [\varepsilon_r \varepsilon_0 \nabla \phi] = e(p - N_a + p_a), \quad (16)$$

where  $\varepsilon_r$  is the relative static dielectric constant of the semiconductor,  $p$  is the density of holes in the valence band,  $N_a$  is the density of acceptors, and  $p_a$  is the density of holes bound to the acceptors (i.e. that  $N_a - p_a$  is the density of ionised acceptor, which are then negatively charged). Within the effective mass approximation, the quantum expression for the density of holes in thermal equilibrium is given by

$$\begin{aligned} p(\mathbf{r}) &= 2 \sum_{v=l,h} \int_{-\infty}^{\infty} \text{LDOS}^{(v)}(\mathbf{r}, E) (1 - f_{\text{FD}}(E)) dE \\ &= \frac{1}{\pi^2} \int_0^{\infty} \int \sum_{v=l,h} \text{Im} \bar{G}^{(v)}(p, z, z, E) (1 - f_{\text{FD}}(E)) dE dp, \end{aligned} \quad (17)$$

where  $f_{\text{FD}}$  is the Fermi-Dirac occupation probability for electrons

$$f_{\text{FD}}(E) = \frac{1}{1 + \exp\left(\frac{E - E_F}{k_B T}\right)}, \quad (18)$$

with the Fermi level  $E_F$ . The factor of 2 in the first line of Eq. (17) corresponds to the spin degeneracy. The steps from the first line to the second simply comes from the invariance by translation in the  $x, y$ -plane and the relation between the LDOS and the imaginary part of the Green's function [8]. The notation  $\sum_{v=l,h}$  in Eq. (17) denotes a sum over light and heavy holes meaning that the LDOS and Green's function are obtained from the Schrödinger equation with the effective mass of the corresponding band. The potential appearing in the Schrödinger equation is given by  $V_v = \delta E_v - e\phi$ , where  $\delta E_v$  is an arbitrary reference for the valence band maximum in the bulk which plays no role as  $\phi$  is defined up to a constant which will be determined by the boundary conditions. Alternatively, the density of holes may be approximated by its semi-classical expression

$$p_{\text{sc}}(\mathbf{r}) = 2 \left[ \frac{m_{\text{eq}} k_B T}{2\pi \hbar^2} \right]^{3/2} \mathcal{F}_{1/2} \left( \frac{V_v(\mathbf{r}) - E_F}{k_B T} \right), \quad (19)$$

where  $m_{\text{eq}}^{3/2} = m_{lh}^{3/2} + m_{hh}^{3/2}$  and  $\mathcal{F}_{1/2}$  is the so-called Fermi integral

$$\mathcal{F}_{1/2}(u) = \frac{2}{\sqrt{\pi}} \int_0^{\infty} \frac{\sqrt{t}}{1 + \exp(t - u)} dt. \quad (20)$$

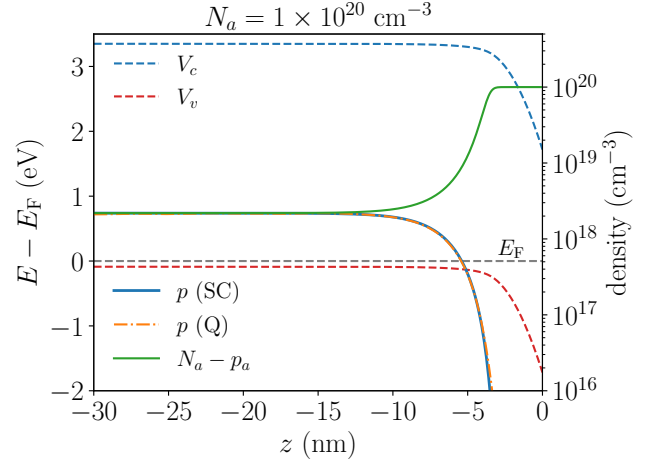

FIG. 1. Conduction and valence band profiles (left axis) and charge carrier densities (right axis) as a function of the  $z$  for GaN with a uniform dopant concentration of  $N_a = 1 \times 10^{20} \text{ cm}^{-3}$ . Blue and red dashed lines: conduction potential and valence potential. The results were obtained by solving self-consistently the Poisson equation with the semi-classical hole density model. The quantum hole density is also shown for the same potential for the sake of comparison.

The two previous expressions originate from the semi-classical approximation of the LDOS,  $\frac{1}{(2\pi)^2} \left[ \frac{2m_{\text{eq}}}{\hbar^2} \right]^{3/2} \sqrt{V_v(\mathbf{r}) - E}$ , in Eq. (17). The density of acceptors  $N_a$  is assumed to be constant in the whole semiconductor and  $p_a$  is given by [9]

$$p_a(\mathbf{r}) = \frac{N_a}{1 + \frac{1}{4} \exp\left(\frac{E_F - V_v(\mathbf{r}) - E_a}{k_B T}\right)}, \quad (21)$$

where  $E_a$  is the activation energy. Solving self-consistently the non-linear Poisson equation using the semi-classical density of holes, we obtain the position dependent electrostatic potential  $\phi$  inside the semiconductor and hence the potentials  $V_c = \delta E_c - e\phi$  and  $V_v = \delta E_v - e\phi$ , with  $\delta E_c - \delta E_v = E_g$ . We choose to work with a homogeneous Neumann boundary condition sufficiently far deep into the bulk, which translate the fact that deep into the semiconductor the electrostatic potential tends to a constant asymptotic value, and with a Dirichlet boundary condition for  $\phi$  at the surface such that the Fermi level is pinned at mid-gap, i.e.,  $e\phi_0 = \frac{\delta E_c + \delta E_v}{2} - E_F$ .

Figure 1 shows the band profiles and the corresponding charge densities for acceptor concentrations  $N_a = 2 \times 10^{20} \text{ cm}^{-3}$  (corresponding to the experimental sample) in GaN at 300 K, obtained with the semi-classical hole density. As a justification for using the semi-classical density, we also show the hole density obtained with the quantum expression for the *same* potential. We observe that the semi-classical and the quantum densities are overall in excellent agreement with only significant deviations close to the interface. The deviation close to the

interface occurs because of the quantum character of the wave functions experiencing the quickly varying potential. However, this is precisely the region in which the hole density can be safely neglected in comparison with the density of ionized acceptors  $N_a - p_a \approx N_a$  which is many orders of magnitude larger than the hole density  $p$ . It is therefore expected that solving the non-linear Poisson equation with the semi-classical or quantum expressions would yield the same electrostatic potential up to a negligible error. This justifies the use of the semi-classical expression instead of the high computationally demanding quantum model. We note that charge neutrality is satisfied in the bulk  $p = N_a - p_a$ .

## II. NUMERICS

### A. Discrete Green's function

The one-dimensional Green's function for a given energy  $E$  and in-plane wave number  $p$  given by Eq. (12) is evaluated numerically as follows. The  $z$ -axis is sliced in thin layers centered on points denoted  $z_{j+1/2}$  and with boundaries  $z_j$  and  $z_{j+1}$  where  $j \in \{1, \dots, N\}$  is an integer. The first interface at  $j = 1$  lies well inside the bulk of the semiconductor  $z_1 = -L$  where the potential is assumed to have reached its asymptotic value, and the last interface  $z_N = L'$  lies in the vacuum where the potential is constant [10]. We do not assume the layers to be regularly spaced in order to have typically a finer grid step where the gradient of the potential is large. Each layer is assumed to be small enough to approximate the local wave-number  $k(z) = \sqrt{2m_c(z)(E - V(z))/\hbar^2 - p^2}$  by a constant within the layer and taken to be its value at the layer's midpoint  $z = z_{j+1/2}$ , i.e.,  $k(z) \approx k(z_{j+1/2}) \equiv k_{j+1/2}$ . We also define the discretized mass  $m_{j+1/2} \equiv m_c(z_{j+1/2})$ . Note that the wave-number may be real or pure imaginary. Consistently with a constant wave-number approximation, the Green's function  $\bar{G}^{(c)}(p, z, z', E)$  is assumed to be the sum of a left and a right propagating or evanescent/growing wave within a layer, i.e.,

$$\bar{G}^{(c)}(z, z') \approx a_j(z') \exp[ik_{j+1/2}(z - z_{j+1})] + b_j(z') \exp[-ik_{j+1/2}(z - z_{j+1})], \quad (22)$$

for  $z_j \leq z \leq z_{j+1}$ . Here and in the following, we will not explicitly write the  $p$  and  $E$  variables for clarity. Note that the amplitudes of the left and right propagating waves depend on the source position  $z'$  which is arbitrary at this stage. The convention used here in the phase of the plane waves in Eq. (22) is made without loss of generality and other conventions may be used up to a redefinition of the amplitudes. We find this convention quite convenient as the Green's function evaluated on the

right boundary of the layer simply becomes

$$\bar{G}^{(c)}(z_{j+1}, z') \approx a_j(z') + b_j(z'). \quad (23)$$

The Green's function in the region  $z < z_1$  inside the bulk of the semiconductor is assumed to take the form of a left propagating or evanescent wave only towards the negative  $z$ -axis,

$$\bar{G}^{(c)}(z, z') = b_0(z') \exp[-ik_{1/2}(z - z_1)] \quad (24)$$

where  $k_{1/2}$  here corresponds to the asymptotic wave number in the bulk. Similarly, in the vacuum, for  $z > z_N$ , we have

$$\bar{G}^{(c)}(z, z') = a_N(z') \exp[ik_{N+1/2}(z - z_N)] \quad (25)$$

where  $k_{N+1/2}$  is the wave number in vacuum. These two last expressions express the fact that we are looking for the Green's function satisfying outgoing radiation conditions. Evaluating the Green's function now amounts to finding the  $2N$  unknown amplitudes  $(b_0(z'), a_1(z'), b_1(z'), \dots, a_{N-1}(z'), b_{N-1}(z'), a_N(z'))$  as a function of the source position  $z'$  which we also discretize on the  $z_j$  grid. In other words, for each value of  $z' = z_k$ , we look for the  $2N$  amplitudes  $(b_{0k}, a_{1k}, b_{1k}, \dots, a_{N-1,k}, b_{N-1,k}, a_{N,k})$  where the second index now refers to the source index, i.e.,  $a_{jk} \equiv a_j(z' = z_k)$  and similarly for the  $b$ -amplitudes. For a given index  $k$ , the amplitudes are linearly related by imposing the continuity of the Green's function and the continuity or jump condition on its derivative divided by the mass at the layer interfaces  $z_j$ . These conditions read for  $1 < j < N$ ,

$$a_{j,k}e_j^+ + b_{j,k}e_j^- - a_{j-1,k} - b_{j-1,k} = 0, \quad (26)$$

$$\frac{i\hbar^2 k_{j+1/2}}{2m_{j+1/2}} (a_{j,k}e_j^+ - b_{j,k}e_j^-) - \frac{i\hbar^2 k_{j-1/2}}{2m_{j-1/2}} (a_{j-1,k} - b_{j-1,k}) = \delta_{jk}, \quad (27)$$

with  $e_j^\pm = \exp[\pm ik_{j+1/2}(z_j - z_{j+1})]$ . Equation (26) is readily obtained by imposing the continuity of the Green's function at the point  $z_j$  from Eq. (22). Let us clarify how to derive the proper continuity or jump condition on the spatial derivative of the Green's function, Eq. (27). Consider first the case where  $z_j \neq 0$ , i.e., the considered point is not at the semiconductor-vacuum interface. Such a point lies inside the semiconductor or outside in the vacuum and we can consider a small interval  $[z_j - \zeta, z_j + \zeta]$  around  $z_j$  with  $\zeta > 0$  intended to tend to 0. For  $\zeta$  small enough the whole interval lies inside the semiconductor or in the vacuum depending on the sign of  $z_j$ , and the effective mass is therefore constant in this interval  $m_c(z) = m_j$ . By integrating Eq. (12) between  $z_j - \zeta$  and  $z_j + \zeta$  we obtain

$$\frac{\hbar^2}{2m_j} \left[ \frac{d\bar{G}^{(c)}}{dz}(z_j + \zeta, z_k) - \frac{d\bar{G}^{(c)}}{dz}(z_j - \zeta, z_k) \right] + \int_{z_j - \zeta}^{z_j + \zeta} \left( E - V_c(z) - \frac{\hbar^2 p^2}{2m_j} \right) \bar{G}^{(c)}(z, z_k) dz = \delta_{jk}, \quad (28)$$

where  $\delta_{jk}$  is the Kronecker delta. When  $\zeta \rightarrow 0$ , the integral in the above equation vanishes and we are left with a continuity or jump condition on the derivative depending on whether  $j \neq k$  or  $j = k$ .

$$\frac{\hbar^2}{2m_j} \left[ \frac{d\bar{G}^{(c)}}{dz}(z_j^+, z_k) - \frac{d\bar{G}^{(c)}}{dz}(z_j^-, z_k) \right] = \delta_{jk}. \quad (29)$$

Consider now the case  $z_j = 0$ . The effective mass now exhibits a jump in the interval  $[z_j - \zeta, z_j + \zeta]$ , from  $m_e$  in the semiconductor to  $m_0$  in the vacuum. Integration of Eq. (12) between  $z_j - \zeta$  and  $z_j + \zeta$  yields

$$\frac{\hbar^2}{2m_0} \frac{d\bar{G}^{(c)}}{dz}(z_j + \zeta, z_k) - \frac{\hbar^2}{2m_e} \frac{d\bar{G}^{(c)}}{dz}(z_j - \zeta, z_k) + \int_{z_j - \zeta}^{z_j + \zeta} \left( E - V_c(z) - \frac{\hbar^2 p^2}{2m_c(z)} \right) \bar{G}^{(c)}(z, z_k) dz = \delta_{jk}, \quad (30)$$

which when  $\zeta \rightarrow 0$  gives

$$\frac{\hbar^2}{2m_0} \frac{d\bar{G}^{(c)}}{dz}(z_j^+, z_k) - \frac{\hbar^2}{2m_e} \frac{d\bar{G}^{(c)}}{dz}(z_j^-, z_k) = \delta_{jk}. \quad (31)$$

Making use of the effective mass evaluated at the  $z_{j \pm 1/2}$ , we see that all cases can thus be summarised as

$$\frac{\hbar^2}{2m_{j+1/2}} \frac{d\bar{G}^{(c)}}{dz}(z_j^+, z_k) - \frac{\hbar^2}{2m_{j-1/2}} \frac{d\bar{G}^{(c)}}{dz}(z_j^-, z_k) = \delta_{jk}. \quad (32)$$

This last equation would also be valid in the more general case of an arbitrary varying effective mass (continuous or not). Inserting Eq. (12) into (32) yields Eq. (27). Equations (26) and (27) are valid for  $1 < j < N$  and thus give  $2(N-2)$  equations. Similar considerations gives 4 additional equations for  $j = 1$  and  $j = N$  for which the expression of the Green's function Eqs. (24) and (25)

must be used. They read for  $j = 1$

$$a_{1,k}e_1^+ + b_{1,k}e_1^- - b_{0,k} = 0 \quad (33)$$

$$\frac{i\hbar^2 k_{3/2}}{2m_{3/2}} (a_{1,k}e_1^+ - b_{1,k}e_1^-) + \frac{i\hbar^2 k_{1/2}}{2m_{1/2}} b_{0,k} = \delta_{1k}, \quad (34)$$

and for  $j = N$

$$a_{N,k} - a_{N-1,k} - b_{N-1,k} = 0 \quad (35)$$

$$\frac{i\hbar^2 k_{N+1/2}}{2m_{N+1/2}} a_{N,k} - \frac{i\hbar^2 k_{N-1/2}}{2m_{N-1/2}} (a_{N-1,k} - b_{N-1,k}) = \delta_{Nk}. \quad (36)$$

Summarizing the  $2N$  linear relations for all values of  $k \in \{1, \dots, N\}$ , we obtain  $2N$  linear systems which we can write in matrix form  $AX = B$  where the matrix  $A$  is given by

$$A = \begin{pmatrix} -1 & e_1^+ & e_1^- & 0 & \dots & \dots & \dots & 0 \\ -\frac{k_{1/2}}{m_{1/2}} & -\frac{k_{3/2}}{m_{3/2}}e_1^+ & \frac{k_{3/2}}{m_{3/2}}e_1^- & 0 & \dots & \dots & \dots & 0 \\ 0 & -1 & -1 & e_2^+ & e_2^- & 0 & \dots & 0 \\ 0 & \frac{k_{3/2}}{m_{3/2}} & -\frac{k_{3/2}}{m_{3/2}} & -\frac{k_{5/2}}{m_{5/2}}e_2^+ & \frac{k_{5/2}}{m_{5/2}}e_2^- & 0 & \dots & 0 \\ \vdots & \vdots & \ddots & \ddots & \ddots & \ddots & \ddots & \vdots \\ 0 & 0 & \dots & -1 & -1 & e_{N-1}^+ & e_{N-1}^- & 0 \\ 0 & 0 & \dots & \frac{k_{N-3/2}}{m_{N-3/2}} & -\frac{k_{N-3/2}}{m_{N-3/2}} & -\frac{k_{N-1/2}}{m_{N-1/2}}e_{N-1}^+ & \frac{k_{N-1/2}}{m_{N-1/2}}e_{N-1}^- & 0 \\ 0 & 0 & \dots & 0 & 0 & -1 & -1 & 1 \\ 0 & 0 & \dots & 0 & 0 & \frac{k_{N-1/2}}{m_{N-1/2}} & -\frac{k_{N-1/2}}{m_{N-1/2}} & -\frac{k_{N+1/2}}{m_{N+1/2}} \end{pmatrix}, \quad (37)$$

and the  $2N \times 2N$  unknown amplitudes and the right-hand side are given by

$$X = \begin{pmatrix} b_{01} & b_{02} & \cdots & b_{0,N-1} & b_{0N} \\ a_{11} & a_{12} & \cdots & a_{1,N-1} & a_{1N} \\ b_{11} & b_{12} & \cdots & b_{1,N-1} & b_{1N} \\ a_{21} & a_{22} & \cdots & a_{2,N-1} & a_{2N} \\ b_{21} & b_{22} & \cdots & b_{2,N-1} & b_{2N} \\ \vdots & \vdots & \ddots & \vdots & \vdots \\ a_{N-2,1} & a_{N-2,2} & \cdots & a_{N-2,N-1} & a_{N-2,N} \\ b_{N-2,1} & b_{N-2,2} & \cdots & b_{N-2,N} & b_{N-2,N} \\ a_{N-1,1} & a_{N-1,2} & \cdots & a_{N-1,N-1} & a_{N-1,N} \\ b_{N-1,1} & b_{N-1,2} & \cdots & b_{N-1,N-1} & b_{N-1,N} \\ a_{N1} & a_{N2} & \cdots & a_{N,N-1} & a_{NN} \end{pmatrix}, \quad B = \frac{2i}{\hbar^2} \begin{pmatrix} 0 & 0 & \cdots & 0 & 0 \\ 1 & 0 & \cdots & 0 & 0 \\ 0 & 0 & \cdots & 0 & 0 \\ 0 & 1 & \cdots & 0 & 0 \\ \vdots & \vdots & \ddots & \vdots & \vdots \\ 0 & 0 & \cdots & 0 & 0 \\ 0 & 0 & \cdots & 1 & 0 \\ 0 & 0 & \cdots & 0 & 0 \\ 0 & 0 & \cdots & 0 & 1 \end{pmatrix}. \quad (38)$$

The left-hand side matrix  $A$  of the linear system being band diagonal, we use an efficient solver for band-diagonal complex-valued matrices, ZGBSV, of the LAPACK library [11].

### B. Discrete non-linear Poisson equation

The one-dimensional non-linear Poisson equation (16) with a constant dielectric constant  $\varepsilon_r$  may be written as

$$-\frac{d^2\phi}{dz^2}(z) = \frac{\rho(z)}{\varepsilon_0\varepsilon_r}, \quad (39)$$

where  $\rho = e(p - N_a + p_a)$  is the charge density. Note that the Poisson equation is non-linear since the charge density depends non-linearly on the electrostatic potential as can be seen from the expressions for  $p_a$ , Eq. (21), and  $p$ , Eq. (17) in the case of the quantum charge density or Eq. (19) for its semi-classical approximation. Given an electrostatic potential, the charge density can thus be computed from these expressions. We consider a regular spatial discretization  $z_j = -L + (j-1)\delta z$  for  $j \in \{1, \dots, N+1\}$ ,  $\delta z = L/N$ , and a three-point finite difference discretization of the second order derivative of  $\phi$ . The Poisson equation can thus be written in vector form as

$$\mathbf{F}(\Phi) = 0, \quad (40)$$

where the unknown electrostatic potential evaluated at the discrete points  $\phi_j \approx \phi(z_j)$ , are gathered in a vector  $\Phi = (\phi_1, \dots, \phi_N)$ , and the components of the vector  $\mathbf{F}$  are given for  $1 < j < N$  by

$$F_j = \frac{\rho_j}{\varepsilon_0\varepsilon_r} + \frac{\phi_{j+1} - 2\phi_j + \phi_{j-1}}{\delta z^2}. \quad (41)$$

For  $j = 1$ , a discrete version of the homogeneous Neumann boundary condition,  $d\phi/dz = 0$ , gives  $\phi_1 = \phi_0$ , hence

$$F_1 = \frac{\rho_1}{\varepsilon_0\varepsilon_r} + \frac{\phi_2 - \phi_1}{\delta z^2}. \quad (42)$$

For  $j = N$ , the Dirichlet boundary condition at the semiconductor-vacuum interface  $\phi_{N+1} = \phi(z = 0) = (\frac{\delta E_c + \delta E_v}{2} - E_F)/e$  yields

$$F_N = \frac{\rho_N}{\varepsilon_0\varepsilon_r} + \frac{\phi(z = 0) - 2\phi_N + \phi_{N-1}}{\delta z^2}. \quad (43)$$

The non-linear discrete Poisson equation (40) can be solved numerically by using the Newton-Raphson method [12]. It consists in solving iteratively

$$\mathbf{J}(\Phi^{(k)})(\Phi^{(k+1)} - \Phi^{(k)}) = -\mathbf{F}(\Phi^{(k)}), \quad (44)$$

where  $\Phi^{(k)}$  is the approximate solution at iteration  $k$ , and  $\mathbf{J} = (\partial F_i / \partial \phi_j)_{i,j \in \{1, \dots, N\}}$  is the Jacobian matrix associated to  $\mathbf{F}$ . Note that in the case of the semi-classical approximation of the charge density, the charge density depends locally on the electrostatic potential. Thus, in this case, the Jacobian matrix is a tridiagonal matrix. The sub- and super-diagonal elements are independent of  $\Phi$  and are readily obtained by differentiation of the second term in the right-hand side of Eqs. (41), (42) and (43) with respect to  $\phi_{j \pm 1}$ . The diagonal elements also depend on the  $\phi_j$  via the  $\rho_j$  and they are evaluated numerically by finite differences.

### C. Numerical parameters

The material parameters which we have used for the numerical simulations are consistent with the parameters representative of the p-doped GaN sample. The band gap was assumed to be  $E_g = 3.437$  eV, the electron effective mass was taken to be  $m_e = 0.21 m_0$ , and the light and heavy hole effective masses  $m_{lh} = 0.14 m_0$ ,  $m_{hh} = 1.87 m_0$ , in unit of the free electron mass  $m_0$ . The acceptor level energy was taken to be  $E_a = 150$  meV above the valence band maximum, and the static relative dielectric constant  $\varepsilon_r = 10.4$ . The nominal dopant concentration was taken to be  $N_a = 1 \times 10^{20} \text{ cm}^{-3}$ , consistent with experimental estimates, and varied between  $N_a = 5 \times 10^{19} \text{ cm}^{-3}$  to  $N_a = 2 \times 10^{20} \text{ cm}^{-3}$  in order to study the sensitivity of the results on the experimental uncertainty on the dopant concentration.

### III. QUANTIZED STATES IN THE BBR OF GAAS PHOTOCATHODES

In this SM section, we come back to the previous attempts to experimentally observe resonant states in the BBR of p-doped semiconductors using low energy photoemission spectroscopy, presented in particular in Refs. [13–15]. First, note that in all of them, the investigated material was p-GaAs, in which the quantization energies are much smaller due to the smaller band bending energy (related to the smaller bandgap) and the much broader BBR, these changes not being compensated by the lighter electron mass. Typically, in Ref. [13], the confined states were evaluated to be around 20 and 100 meV (for the higher and lower energy states, respectively) below the bulk conduction band minimum. The configuration in which we were able to best observe the resonant states in p-GaN was the one in which the sample was excited above the highest resonant state but below the GaN bandgap. This way, we could see the signature of resonant states without being masked by the larger contribution from  $\Gamma$  electrons accumulated in the bulk conduction band minimum and relaxing down in the BBR. This situation is much more difficult to achieve in GaAs, and we believe that in studies of photoemission from the BBR in GaAs, the resonant states contribution could not be distinguished from the  $\Gamma$  contribution.

In Ref. [13], excitation energies are chosen around the GaAs bandgap. The authors interpret peak I0 in their Figures 1 and 3 as electrons coming from the second (high-energy) resonant state in the BBR. However, they only observe this peak when the bulk conduction band is populated (either directly from the valence band maximum or from the acceptor levels, the acceptors activation energy being of the order of 20 meV). Considering the commonly accepted EDC interpretation presented on GaAs by Drouhin et al. [16], this I0 peak would more reasonably correspond to the  $\Gamma$  contribution. Looking at the evolution of the  $\Gamma$  contribution in EDCs from room temperature to 120K in [16], we can expect such narrow and

high energy  $\Gamma$  contribution at 4.2K as in Figures 1 and 3 of Ref. [13]. They also do not observe the lower quantized state as their other observed lines are attributed to LO-phonon replicas. When exciting with energies higher than the bandgap, although it is highly probable that the energy relaxation of the  $\Gamma$  electrons entering the BBR is affected by the presence of resonant states, the effect on the resulting EDC is not obvious, as attested by the curves at room temperature and 120K in Ref. [16] where the  $\Gamma$  peak extends much lower in energy than the high energy resonant state.

In the works of Ref. [14] (Figure 1), the photoemission experiments are performed at room temperature with above bandgap excitation. The EDC are dominated by the  $\Gamma$  contribution, as well as by the first lateral valley contribution for higher excitation energies. These peaks have a high energy threshold at the bulk position of the corresponding band minimum and extend to lower energies due to relaxation in the BBR [16]. This extension to lower energies is mistakenly taken for an accumulation in the confined states of the BBR. Again, note that the shift of the  $\Gamma$  contribution to lower energies strongly depends on temperature [13, 16], which is not consistent with the interpretation given in Ref. [14].

In Ref. [15] (Figure 5), the photoemission current excited with a laser energy of 1.58eV, i.e. 0.16 eV above the GaAs bandgap, is monitored as a function of the workfunction change during NEA degradation process. The authors in Ref. [15] interpret the peak of a broad change in the derivative of the photocurrent as the position of the higher quantized energy level in the BBR. It is hard to see this change as a measurement of a quantized state as one would expect a rather sharp transition when the workfunction level crosses the quantized state. We are rather in the same situation as in Ref. [16] Figure 11, with above bandgap excitation like in Ref. [15], where the low energy part of the EDC shows two components, one due to the direct  $\Gamma$  contribution, the other due to  $\Gamma$  electrons relaxing down the BBR with no defined structure.

- 
- [1] C. Weisbuch and B. Vinter, *Quantum Semiconductor Structures* (Academic Press, San Diego, 1991).
  - [2] G. Bastard, Superlattice band structure in the envelope-function approximation, *Phys. Rev. B* **24**, 5693 (1981).
  - [3] J.-M. Lévy-Leblond, Position-dependent effective mass and Galilean invariance, *Phys. Rev. A* **52**, 1845 (1995).
  - [4] G. T. Einevoll and L. J. Sham, Boundary conditions for envelope functions at interfaces between dissimilar materials, *Phys. Rev. B* **49**, 10533 (1994).
  - [5] A. G. Zhuravlev, A. S. Romanov, and V. L. Alperovich, Photon-enhanced thermionic emission from p-GaAs with nonequilibrium Cs overlayers, *Appl. Phys. Lett.* **105**, 251602 (2014).
  - [6] E. Akkermans and G. Montambaux, *Mesoscopic Physics of Electrons and Photons* (Cambridge University Press, 2007).
  - [7] M. Born and E. Wolf, *Principles of Optics: Electromagnetic Theory of Propagation, Interference and Diffraction of Light*, 7th ed. (Cambridge University Press, Cambridge, 1999).
  - [8] Note the sign difference for the valence band compared with Eq. (15). This comes from the fact that the effective mass Schrödinger operator for valence band is a negative operator.
  - [9] J. Singh, *Electronic and Optoelectronic Properties of Semiconductor Structures* (Cambridge University Press, 2003).
  - [10] In fact, it suffices to take  $L' = 0$ , at the semiconductor surface, since the general form of the Green's function for  $z > 0$  in a region of constant potential is known analytically.

- cally.
- [11] LAPACK – Linear Algebra PACKage, <https://netlib.org/lapack/>.
  - [12] W. H. Press, S. A. Teukolsky, W. T. Vetterling, and B. P. Flannery, *Numerical Recipes*, 3rd ed. (Cambridge University Press, Cambridge, 2007).
  - [13] D. Orlov, V. Andreev, and A. Terekhov, Elastic and inelastic tunneling of photoelectrons from the dimensional quantization band at a  $p + -\text{GaAs} - (\text{Cs}, \text{O})$  interface into vacuum, *JETP Lett.* **71**, 151–154 (2000).
  - [14] V. L. Korotkikh, A. L. Musatov, and V. D. Shadrin, Influence of size-effect quantization of energy levels in semiconductors on the photoelectron emission, *JETP Lett.* **27**, 652 (1978).
  - [15] X. Jin, Analysis of electron emission from  $\text{GaAs}(\text{Cs}, \text{O})$  by low energy electron microscopy, *Japanese Journal of Applied Physics* **54**, 101201 (2015).
  - [16] H.-J. Drouhin, C. Hermann, and G. Lampel, Photoemission from activated gallium arsenide. I. Very-high-resolution energy distribution curves, *Phys. Rev. B* **31**, 3859 (1985).
